# Supplementary material for: Lifted Neural Networks
Source: arXiv:1805.01532 source file (2018-06-21)
Supplement: Supplementary file 1 [file non_convex_appendix.tex]

\section{Equations for the subproblems}
\paragraph{Updating the first layer weight variables}
Here we provide additional details of updating the first layer weight variables.  In particular, if the activation function in the first layer is a ReLU, then the update for the first layer weight variables becomes
\begin{align*}
&(W, U_0, b_0) = \displaystyle\arg\min_{W,U_{0},b_{0}} \\
& \: \lambda \|
\sum_{j=0}^{T-1} \|H_{1,j} - 
\begin{pmatrix}
H_{1,j-1} & X_{j} & \ones
\end{pmatrix}
\begin{pmatrix}
W \\
U_0 \\
b_0^{T}
\end{pmatrix}
\|_{F}^{2}\\
&+ \rho_0 \|U_{0}\|_F^2
+\rho_2 \|W\|_F^2
\end{align*}

\paragraph{Updating the second layer weight variables}
Here we provide additional details of updating the second layer weight variables.  In particular, if there is no activation in the second layer and the objective loss is a frobenius norm squared (a regression problem), then the update for the second layer weight variables becomes

\begin{align*}
(U_{1}, b_{1}) = &\arg \displaystyle\min_{U_{1}, b_{1}} \sum_{j=0}^{T-1} \|Y_{j} - 
\begin{pmatrix}
H_{1,j} & \ones
\end{pmatrix}
\begin{pmatrix}
U_{1} \\
b_{1}^{T}
\end{pmatrix}
\|_{F}^{2} &+ \rho_{1}\|U_{1}\|_{F}^{2}
\end{align*}

\paragraph{Updating the state variables}
Here we provide additional details of updating each state in the hidden layer.  When the activation functions are ReLU's and the objective loss is a frobenius norm squared (a regression problem) then the update for each hidden state becomes
\begin{align*}
&H_{1,j} = \arg \displaystyle\min_{H \ge 0} \lambda \|H - X_{j}U_{0} - \ones b_{0}^{T} - H_{1,j-1}W\|_{F}^{2}+\\
& \lambda \|H_{1,j+1} - X_{j+1}U_{0} - \ones b_{0}^{T} - H W\|_{F}^{2} + \|Y_j - H U_0\|_{F}^{2}
\end{align*}
